# Supplementary material for: Non-equilibrium conductivity at quantum critical points
Source: arXiv:1312.4432 source file (2014-01-14)
Supplement: Supplementary file 1 [file Supplementary.pdf]

.

# Non-equilibrium conductivity at quantum critical points - Supplementary materials

A.M. Berridge[1] and A.G. Green[1]

[1]London Centre for Nanotechnology, University College London, 17-19 Gordon St, London, WC1H 0AH, UK

(Dated: December 6, 2013)

We present supplementary materials for our paper "Non-equilibrium conductivity at quantum critical points". These include calculational methods and extended explanations that were not included in the main paper in order to maintain narrative flow. Firstly we consider the scattering integral and show how we derive its highly antisymetrically-boosted form. We then show explicitly how spatial gradients in the Boltzmann equation can be replaced by a sink term. This sink is given in terms of a zero-mode of the scattering integral. We present an argument for the form of this zero-mode. The variational solution is concluded by taking moments of the Boltzmann equation. We then outline the expansion around a thermal distribution, taking time to detail the derivation of the linearised scattering integrals. This expansion does not converge.

## I. EFFECTIVE FIELD THEORY

We study the continuum field theory of the Bose-Hubbard model at integer fillings, minimally coupled to an electric field. The imaginary-time action for this model takes the form[4]

$$\mathcal{S} = \int d\tau d\mathbf{x} \left[ |\partial_\tau \phi|^2 + |(\partial_{\mathbf{x}} + i\mathbf{A})\,\phi|^2 + m^2 |\phi|^2 + \frac{u}{3!}|\phi|^4 \right], \tag{1}$$

where $\phi$ is a complex scalar field, $\mathbf{A}$ a vector potential representing a uniform electric field, $m$ the effective mass and $u$ the interaction. At the critical coupling, the effective mass and interaction strength may be evaluated within an $\epsilon$-expansion about 3 spatial dimensions with the results[4] $m^2 = \epsilon \frac{4\phi^2 T^2}{15}$ and $u = \frac{24\pi^2}{5}\epsilon$. The $\epsilon$-expansion allows the interaction to be treated perturbatively. The quadratic part of Eq.(1) is a Klein-Gordon model. We follow Damle and Sachdev[4] and study a Boltzmann equation for the occupation of positively and negatively charges normal modes of this model under the application of a strong electric field (see section V).

## II. HEAT FLOW

### A. The sink term and effective temperature

In order to reach a steady-state solution the energy produced by Joule heating and the particle production by the source term must be compensated by a sink term. This is achieved by introducing a heat flow to a bath at the system edge[1]. Conservation of energy means that the system has an infinite thermal conductivity, therefore the temperature gradients required to carry this heat can be arbitrarily small. We find a homogenoeus sink term which captures the effect of the heat flow. Due to the infinite thermal conductivity of the model the rate limiting step in dissipating energy is not the rate which it can be transported to the system edge but the rate which it can be scattered into the heat-carrying section of the distribution. This is governed by the scattering processes rather than sample geometry and so the sink is universal.

#### 1. Heat flow

A heat-flow to the sample edge is set up by expanding the distribution function in gradients in the direction transverse to the electric field,

$$f^{\pm}_{\mathbf{k}}(y) \;=\; f^{\pm}_{\mathbf{k}} + h^{(0),\pm}_{\mathbf{k}} + y h^{(1),\pm}_{\mathbf{k}} + \frac{y^2}{2} h^{(2),\pm}_{\mathbf{k}}, \tag{2}$$

where $y$ is the direction transverse to the field. Here $f^{\pm}_{\mathbf{k}}$ is the distribution which we expand around, with some effective temperature $T_{eff}$, and the $h_{\mathbf{k}}$ are deviations from this distribution. Substituting into the Boltzmann equation

$$(\mp\mathbf{E}\cdot\partial_{\mathbf{k}} + \mathbf{v}\cdot\partial_{\mathbf{r}})\, f^{\pm}_{\mathbf{k}} \;=\; S^{\pm}_{\mathbf{k}}[f^{\pm}_{\mathbf{q}}] + g^{source}_{\mathbf{k}}, \tag{3}$$

and equating powers of $y$ we find:

$$\begin{aligned} y^0 : &\quad \mp\mathbf{E}\cdot\partial_{\mathbf{k}}(f^{(0),\pm}_{\mathbf{k}} + h^{(0),\pm}_{\mathbf{k}}) + v^y h^{(1),\pm}_{\mathbf{k}} \\ &\quad = S^{\pm}_{\mathbf{k}}[f^{\pm}_{\mathbf{q}}] + \mathcal{S}_{\mathbf{k},\mathbf{q}} h^{(0),\pm}_{\mathbf{q}} + g^{source}_{\mathbf{k}}, \\ y^1 : &\quad \mp\mathbf{E}\cdot\partial_{\mathbf{k}} h^{(1),\pm}_{\mathbf{k}} + v^y h^{(2),\pm}_{\mathbf{k}} = \mathcal{S}_{\mathbf{k},\mathbf{q}} h^{(1),\pm}_{\mathbf{q}}, \end{aligned} \tag{4}$$

where $v^y = \frac{\mathbf{k}\cdot\hat{\mathbf{y}}}{|k|}$ and $\mathcal{S}_{\mathbf{k},\mathbf{q}}$ is the linearised scattering integral. We may now solve for the homogeneous component in terms of $h^{(2)}_{\mathbf{k}}$. We will then use properties of the scattering integral to solve for this in terms of zero-modes. For notational simplicity we treat $S^{\pm}_{\mathbf{k}}[f^{\pm}_{\mathbf{q}}]$ as an additional source term $\tilde{g}^{source,\pm}_{\mathbf{k}} = g^{source}_{\mathbf{k}} + S^{\pm}_{\mathbf{k}}[f^{\pm}_{\mathbf{q}}]$. Substituting we find:

$$
\begin{aligned}
h_{\mathbf{k}}^{(1),\pm} &= \left(1-\mathcal{S}^{-1}\mp\mathbf{E}\cdot\partial_{\mathbf{q}}\right)^{-1}_{\mathbf{k},\mathbf{q}}\mathcal{S}^{-1}_{\mathbf{q},\mathbf{p}}v^y h_{\mathbf{p}}^{(2),\pm} \\
&\simeq \mathcal{S}^{-1}_{\mathbf{k},\mathbf{q}}v^y h_{\mathbf{q}}^{(2),\pm}, \\
h_{\mathbf{k}}^{(0),\pm} &= \left(1-\mathcal{S}^{-1}\mp\mathbf{E}\cdot\partial_{\mathbf{q}}\right)^{-1}_{\mathbf{k},\mathbf{q}}\mathcal{S}^{-1}_{\mathbf{q},\mathbf{p}}\mathbf{E}\cdot\partial_{\mathbf{p}}f_{\mathbf{p}}^{(0),\pm}-\left(1-\mathcal{S}^{-1}\mp\mathbf{E}\cdot\partial_{\mathbf{q}}\right)^{-1}_{\mathbf{k},\mathbf{q}}\mathcal{S}^{-1}_{\mathbf{q},\mathbf{p}}\,\tilde{g}_{\mathbf{p}}^{source,\pm} \\
&\quad+\left(1-\mathcal{S}^{-1}\mp\mathbf{E}\cdot\partial_{\mathbf{q}}\right)^{-1}_{\mathbf{k},\mathbf{q}}\mathcal{S}^{-1}_{\mathbf{q},\mathbf{p}}v^y\left(1-\mathcal{S}^{-1}\mp\mathbf{E}\cdot\partial_{\mathbf{l}}\right)^{-1}_{\mathbf{p},\mathbf{l}}\mathcal{S}^{-1}_{\mathbf{l},\mathbf{m}}v^y h_{\mathbf{m}}^{(2),\pm} \\
&\simeq \left(1-\mathcal{S}^{-1}\mp\mathbf{E}\cdot\partial_{\mathbf{q}}\right)^{-1}_{\mathbf{k},\mathbf{q}}\mathcal{S}^{-1}_{\mathbf{q},\mathbf{p}}\mp\mathbf{E}\cdot\partial_{\mathbf{p}}f_{\mathbf{p}}^{(0),\pm}-\mathcal{S}^{-1}_{\mathbf{k},\mathbf{q}}\tilde{g}_{\mathbf{q}}^{source,\pm}+\mathcal{S}^{-1}_{\mathbf{k},\mathbf{q}}v^y\mathcal{S}^{-1}_{\mathbf{q},\mathbf{p}}v^y h_{\mathbf{p}}^{(2),\pm}.
\end{aligned}
\tag{5}
$$

Expanding $h_{\mathbf{k}}^{(0)}$ to leading order in $\mathcal{S}^{-1}$ leads to a homogeneous component of the distribution function,

$$
\begin{aligned}
f_{\mathbf{k}}^{\pm} &= \left(1_{\mathbf{k},\mathbf{q}}+\mathcal{S}^{-1}_{\mathbf{k},\mathbf{q}}\mp\mathbf{E}\cdot\partial_{\mathbf{q}}\right)f_{\mathbf{q}}^{(0),\pm}-\mathcal{S}^{-1}_{\mathbf{k},\mathbf{q}}\tilde{g}_{\mathbf{q}}^{source,\pm}+\mathcal{S}^{-1}_{\mathbf{k},\mathbf{q}}v^y\mathcal{S}^{-1}_{\mathbf{q},\mathbf{p}}v^y h_{\mathbf{p}}^{(2),\pm} \\
&= f_{\mathbf{k}}^{0,\pm}+\mathcal{S}^{-1}_{\mathbf{k},\mathbf{q}}\left(\mp\mathbf{E}\cdot\partial_{\mathbf{q}}f_{\mathbf{q}}^{(0),\pm}-\tilde{g}_{\mathbf{q}}^{source,\pm}+\underbrace{v^y\mathcal{S}^{-1}_{\mathbf{q},\mathbf{p}}v^y h_{\mathbf{p}}^{(2),\pm}}_{g_{\mathbf{q}}^{sink}}\right).
\end{aligned}
\tag{6}
$$

We note that the final contribution to the homogeneous distribution is actually the scattering integral acting on the coefficient of the leading-order, y-linear term. This part of the distribution function represents the heat-current that builds linearly across the sample. This term appears in the Boltzmann equation as $v^y\partial_y(yh_{\mathbf{k}}^{(1)}) = v^y\mathcal{S}^{-1}_{\mathbf{k},\mathbf{q}}v^y h_{\mathbf{q}}^{(2)}$. The sink therefore represents scattering into the heat current.

### 2. Heat sink

We now find a homogeneous solution by introducing a sink term. We have shown that $-v^y\mathcal{S}^{-1}_{\mathbf{k},\mathbf{q}}v^y h_{\mathbf{q}}^{(2)}$ appears in the Boltzmann equation in the same way as $g_{\mathbf{k}}^{source}$ and will therefore be our sink term.

$$
\mp\mathbf{E}\cdot\partial_{\mathbf{k}}f_{\mathbf{k}}^{\pm} = \mathcal{S}_{\mathbf{k},\mathbf{q}}f_{\mathbf{q}}^{\pm}+g_{\mathbf{k}}^{source,\pm}-v_{\mathbf{k}}^y\mathcal{S}^{-1}_{\mathbf{k},\mathbf{q}}v_{\mathbf{q}}^y h_{\mathbf{q}}^{(2),\pm}
\tag{7}
$$

Using the properties of the scattering integral we can rewrite $g_{\mathbf{k}}^{sink} = v_{\mathbf{k}}^y\mathcal{S}^{-1}_{\mathbf{k},\mathbf{q}}v_{\mathbf{q}}^y h_{\mathbf{q}}^{(2)}$ independently of the unknown term $h_{\mathbf{k}}^{(2)}$. Rearranging we have $\mathcal{S}_{\mathbf{k},\mathbf{q}}\left(g_{\mathbf{q}}^{sink}/v_{\mathbf{q}}^y\right) = v_{\mathbf{k}}^y h_{\mathbf{k}}^{(2)}$. Considering the symmetry of the various terms $v_{\mathbf{k}}^y$ has the form $\hat{\mathbf{y}}\cdot\mathbf{k}/|k|$ and the linearised scattering integral is therefore particle-hole symmetric, $k$-antisymmetric[2]. This scattering integral has a zero mode related to the infinite thermal conductivity of the model. The inverse of the scattering integral is dominated by this zero-mode and the sink term is therfore given by,

$$
g_{\mathbf{k}}^{sink,\pm} = \alpha v_{\mathbf{k}}^y h_{\mathbf{k}}^{\pm},
\tag{8}
$$

where $h_{\mathbf{k}}^{\pm}$ is the momentum zero-mode and $\alpha$ is a constant to be determined. Particles are scattered into the zero mode where they are transported to the edge of the system without further scattering. Note that the existence of the zero-mode is fixed by the symmetries of the scattering integral. This general form for the sink is universal, although the exact form of the zero-mode depends upon the distribution we expand around. The form of this zero mode is calculated in the next section.

The rate-limiting step in dissipating heat is the scattering of particles into the heat-carrying mode, which then transports the heat away arbitrarily quickly. In this way the solution becomes universal, and independent of sample details. However, we still require a way to set the remaining parameters in the sink - $\alpha$, the effective temperature $\tilde{T}_{eff}$, and the boost velocity $v$, which appear in the zero-mode. This is achieved by taking moments of the Boltzmann equation as described in section (IV).

## III. ZERO MODES

In order to calculate the explicit form of the sink term we now consider the zero modes of the scattering integral which will be described in section (V).

The zero modes of the scattering integral linearised about a thermal distribution are easily found from conservation laws. For the zero-mode relating to energy conservation we know that $\mathcal{S}[f^T] = \mathcal{S}[f^{T+\Delta T}] = \mathcal{S}[f^T] + \Delta T\,\delta\mathcal{S}\,\partial_T f^T$, with $\delta\mathcal{S}$ the linearised scattering integral. Since both $\mathcal{S}[f^T]$ and $\mathcal{S}[f^{T+\Delta T}]$ equal zero this leads to $\delta\mathcal{S}\partial_T f^T = 0$, therefore $h_{\mathbf{k}}^E = \partial_T f^T$ is a zero-mode of the linearised scattering integral $\delta\mathcal{S}$. The zero modes of the scattering integral acting on the antisymmetrically boosted distribution must be calculated differently as the scattering integral acting on the distribution is not zero. We present a derivation that also works in the equilib-

rium case.

We are interested in the zero mode related to heat transport. A heat current is carried by a particle-hole symmetric distortion of the distribution function in the direction transverse to the direction of the electic field. We consider the solution of the Boltzmann equation with a temperature gradient.

$$f^v(\nabla T) \;=\; f^v + \mathbf{x}\cdot\frac{\nabla\mathbf{T}}{T}\partial_T f^v + \delta f^h, \qquad (9)$$

where $\delta f^h$ is the heat current response. Substituting this into the Boltzmann equation gives the homogeneous solution:

$$\mathbf{E}\cdot\partial_{\mathbf{k}} f^v_{\mathbf{k}} \;=\; g^{source}_{\mathbf{k}} + g^{sink}_{\mathbf{k}} + \mathcal{S}_{\mathbf{k}}[f^v], \qquad (10)$$

plus the response to the temperature gradient:

$$\begin{aligned}\mathbf{v}\cdot\partial_{\mathbf{x}}\left(\mathbf{x}\cdot\frac{\nabla\mathbf{T}}{T}\partial_T f^v_{\mathbf{k}}\right) &= \mathcal{S}_{\mathbf{k},\mathbf{q}}\delta f^h_{\mathbf{q}},\\ -\mathbf{k}\cdot\frac{\nabla\mathbf{T}}{T}\partial_\epsilon f^v_{\mathbf{k}} &= \mathcal{S}_{\mathbf{k},\mathbf{q}}\delta f^h_{\mathbf{q}},\\ \delta f^h_{\mathbf{k}} &= -\mathcal{S}^{-1}_{\mathbf{k},\mathbf{q}}\left(\mathbf{q}\cdot\frac{\nabla\mathbf{T}}{T}\partial_\epsilon f^v_{\mathbf{q}}\right).\end{aligned} \qquad (11)$$

We expect that there will be a very large heat current for even a small temperature gradient and therefore $\mathbf{k}\cdot\frac{\nabla\mathbf{T}}{T}\partial_\epsilon f_v$ must be nearly a zero-mode. In thermal equilibrium this gives the same zero-mode as identified previously. For the boosted thermal distribution it is given explicitly by

$$h^+_{\mathbf{k}} \;=\; -\mathbf{k}\cdot\mathbf{u}\frac{(1+\frac{\mathbf{v}\cdot\mathbf{k}}{k})}{T\sqrt{1-v^2}}\partial_\epsilon f_v. \qquad (12)$$

## IV. TAKING MOMENTS OF THE BOLTZMANN EQUATION

There are three undetermined constants in our solution, the antisymmetric boost velocity $v$, the effective temperature prefactor $\tilde{T}_{eff}$ and the over all prefactor of the sink term $\alpha$. In order to fix these we will take three moments of the Boltzmann equation. Two of these represent number and energy conservation and reveal the balance of particle production/destruction by the source and sink and Joule heating. In these terms the scattering integral vanishes due to conservation of number and energy in the scattering processes. The third moment encodes the effect of scattering on the solution.

### A. Source and sink terms

We require explicit forms for the source and sink terms. The form of the source is calculated in Ref.(3). We will use a symmetrised version of this result? :

$$g^{source}_{\mathbf{k}} \;=\; \frac{\pi}{4}\sqrt{E}e^{-\pi k^2/E}. \qquad (13)$$

As calculated in section (II) the sink term is given by $g^{sink}_{\mathbf{k}} = \alpha v^y h_{\mathbf{k}}$ where $v^y = \hat{\mathbf{y}}\cdot\hat{\mathbf{k}}$ with $\mathbf{y}\perp\mathbf{v}$. Combined with Eq.(12) this gives:

$$g^{sink}_{\mathbf{k}} \;=\; \alpha v^y v^y\frac{k(1-vc)}{T_{eff}\sqrt{1-v^2}}\partial_\epsilon f^T\left(\frac{k(1-vc)}{T_{eff}\sqrt{1-v^2}}\right) \qquad (14)$$

where $c$ represents the full angular dependence of the product $\mathbf{v}\cdot\mathbf{k}$.

### B. Moments of the Boltzmann equation

In order to obtain three equations to fix the three parameters of the solution we will take moments of the Boltzmann equation. Firstly we sum the Boltzmann equation over particle species. The first moment is taken by integrating over $\mathbf{k}$. This represents conservation of number. The second by multiplying by $\epsilon_{\mathbf{k}}$ before integrating, representing conservation of energy. And the third by multiplying by $\epsilon^2_{\mathbf{k}}$ before integrating:

$$\sum_{\sigma=\pm}\mathbf{E}\cdot\int_{\mathbf{k}}\partial_{\mathbf{k}} f^\pm_{\mathbf{k}} \;=\; 2\int_{\mathbf{k}} g^{source}_{\mathbf{k}} - 2\int_{\mathbf{k}} g^{sink}_{\mathbf{k}}, \qquad (15)$$

$$\sum_{\sigma=\pm}\mathbf{E}\cdot\int_{\mathbf{k}}\epsilon_{\mathbf{k}}\partial_{\mathbf{k}} f^\pm_{\mathbf{k}} \;=\; 2\int_{\mathbf{k}}\epsilon_{\mathbf{k}} g^{source}_{\mathbf{k}} - 2\int_{\mathbf{k}}\epsilon_{\mathbf{k}} g^{sink}_{\mathbf{k}}, \qquad (16)$$

$$\begin{aligned}\sum_{\sigma=\pm}\mathbf{E}\cdot\int_{\mathbf{k}}\epsilon^2_{\mathbf{k}}\partial_{\mathbf{k}} f^\pm_{\mathbf{k}} &= \sum_{\sigma=\pm}\int_{\mathbf{k}}\epsilon^2_{\mathbf{k}}\mathcal{S}_{\mathbf{k}}[f^\sigma_{\mathbf{q}}]\\ &\quad +2\int_{\mathbf{k}}\epsilon^2_{\mathbf{k}} g^{source}_{\mathbf{k}} - 2\int_{\mathbf{k}}\epsilon^2_{\mathbf{k}} g^{sink}_{\mathbf{k}}.\end{aligned} \qquad (17)$$

Here the factors of 2 come from the sum over species and the scattering term integrates to zero in the first two equations since it conserves number and energy by construction.

*First moment* — The left hand side of Eq.(15) gives 0 as it is a total derivative, substituting Eqns.(13,14) on the right hand side gives:

$$\begin{aligned}0 &= \frac{\pi}{2}E^2\\ &\quad +\alpha T^3_{eff}24\zeta(3)\pi\frac{\frac{v}{1-v^2}-\mathrm{ArcTanh}(v)}{v^3}(1-v^2)^{3/2}\\ &\simeq \frac{\pi}{2}E^2 + \alpha T^3_{eff}24\pi\zeta(3)\sqrt{2\delta v},\\ \alpha &\simeq -\frac{1}{48\zeta(3)}\frac{\sqrt{E}}{\tilde{T}^3_{eff}}\frac{1}{\sqrt{2\delta v}}.\end{aligned} \qquad (18)$$

Where $\delta v = 1 - v$, which we assume to be small.

*Second moment* — The left hand side of Eq.(16) represents Joule heating, $-\sum_{\sigma=\mp}\mathbf{E}\cdot\int d\mathbf{k}k\partial_{\mathbf{k}}f^{\pm}=\sigma_E E^2$ where $\sigma_E$ is the electrical conductivity. Substituting Eqns.(13,14) on the right hand side gives:

$$-ET^3\frac{8\pi v}{3\sqrt{1-v^2}}6\zeta(3) \;=\; E^{5/2}+\alpha T^4\frac{8\pi}{3}\frac{4\pi^4}{15}. \quad (19)$$

*Third moment* — The third moment, Eqn.(17) contains an integral over the scattering term which is non-zero, we use the high-boost approximation given in section (VI). This moment is given by:

$$-ET^4\frac{16\pi v}{3}\frac{1}{(1-v^2)}\frac{4\pi^4}{15} \;=\; -2\frac{2\pi^3\epsilon^2}{75}\frac{4\pi}{3}\frac{3+v^2}{1-v^2}\frac{\pi^4}{15}T^6+\frac{6E^3}{8}+\alpha T^5\frac{8\pi}{3}120\zeta(5)\frac{1}{\sqrt{1-v^2}}. \quad (20)$$

These three equations need to be solved simultaneously in order to fix the parameters of the distribution. We do so after expanding in the limit $\delta v \ll 1$. This gives the following values for the parameters of the variational ansatz:

$$\begin{aligned}\tilde{T}_{eff} &= 0.2,\\ \alpha &= 8.14,\\ v &= 0.96. \end{aligned} \quad (21)$$

As $v$ is close to one we are in the high-boost limit and both the small $\delta v$ approximation and approximation to the scattering integral are self-consistent. We may also solve the equations for the exact $v$ numerically, finding a result in good agreement with the expansion in $\delta v$.

## V. THE SCATTERING INTEGRAL

The scattering integral as calculated in the $\epsilon$-expansion is given by[4]:

$$\begin{aligned} S^{\pm}_{\mathbf{k}}[f^{\pm}_{\mathbf{q}}] &= -\frac{2u_0^2}{9}\int\frac{d\mathbf{k}_1}{(2\pi)^d}\frac{d\mathbf{k}_2}{(2\pi)^d}\frac{d\mathbf{k}_3}{(2\pi)^d}\frac{(2\pi)^{d+1}}{16kk_1k_2k_3}\delta\left(\mathbf{k}+\mathbf{k}_1-\mathbf{k}_2-\mathbf{k}_3\right)\delta\left(k+k_1-k_2-k_3\right)\\ &\quad\times\left(\mathcal{F}^{out}_{\pm}-\mathcal{F}^{in}_{\mp}\right),\\ \mathcal{F}^{out}_{\pm} &= \underbrace{2f^{\pm}_{\mathbf{k}}f^{\mp}_{\mathbf{k_1}}\left[1+f^{\pm}_{\mathbf{k_2}}\right]\left[1+f^{\mp}_{\mathbf{k_3}}\right]}_{particle-hole}+\underbrace{f^{\pm}_{\mathbf{k}}f^{\pm}_{\mathbf{k_1}}\left[1+f^{\pm}_{\mathbf{k_2}}\right]\left[1+f^{\pm}_{\mathbf{k_3}}\right]}_{particle-particle}, \end{aligned} \quad (22)$$

where the in-scattering term follows by interchanging $f^{\pm}$ and $1+f^{\pm}$. At the critical point the coupling has the value $\frac{2u_0^2}{9}=\frac{128\pi^4\epsilon^2}{25}$. The delta-functions enforce energy and momentum conservation. The scattering integral consists of contributions from in- and out-scattering into a state labelled by $\mathbf{k}$ and has terms corresponding to particle-particle and particle-hole scattering.

When evaluated for a thermal distribution this integral gives zero by definition. We need to evaluate it for non-thermal distributions. In section VII we linearise the distribution about a thermal distribution in order to expand about this state. In section VI we consider an antisymmetric highly-boosted distribution, which turns out to be a much better approximation. The scattering integral calculated in this limit takes a particularly simple form.

## VI. HIGH-BOOST APPROXIMATION

We discuss a form for the scattering integral valid in the highly-boosted limit. We argue that in-scattering can be neglected due to a phase-space argument and that the out-scattering reduces to a simple form. This is very similar to the appearance of the scattering integral in the $1/N$ expansion[3], which will be reflected in the solution for the distribution function.

It is difficult to evaluate the scattering integral for an arbitrary distribution, but we are helped by the form of the Lorentz-boosted distribution. The particle-particle scattering terms of the scattering integral give zero when acting on a boosted distribution due to Lorentz invariance[2]. However as particles and holes are boosted in opposite directions by the electric field the particle-hole scattering terms are not zero. In order to evaluate the particle-hole scattering we use the following approxi-

mation scheme, valid in the highly-boosted limit. The particle-hole scattering term contains contributions from in- and out-scattering:

$$S^{ph}_{\mathbf{k}}[f^{\pm}_{\mathbf{q}}] = -\frac{2u_0^2}{9}\frac{1}{(2\pi)^{2d-1}}\frac{1}{k}\int\frac{d\mathbf{k}_1}{2k_1}\frac{d\mathbf{k}_2}{2k_2}\frac{d\mathbf{k}_3}{2k_3}\delta\left(\mathbf{k}+\mathbf{k}_1-\mathbf{k}_2-\mathbf{k}_3\right)\delta\left(k+k_1-k_2-k_3\right) \times\left(\underbrace{f^{+}_{\mathbf{k}}f^{-}_{\mathbf{k}_1}\left(1+f^{+}_{\mathbf{k}_3}\right)\left(1+f^{-}_{\mathbf{k}_4}\right)}_{OUT}-\underbrace{\left(1+f^{+}_{\mathbf{k}}\right)\left(1+f^{-}_{\mathbf{k}_1}\right)f^{+}_{\mathbf{k}_2}f^{-}_{\mathbf{k}_3}}_{IN}\right). \quad (23)$$

As our distribution is highly elongated we assume that out scattering is dominated by scattering into empty states and therefore take $1+f_{\mathbf{k}}\to 1$ in the scattering integral:

$$S^{ph}_{\mathbf{k}}[f^{\pm}_{\mathbf{q}}] = -\frac{2u_0^2}{9}\frac{1}{(2\pi)^{2d-1}}\frac{1}{k}\int\frac{d\mathbf{k}_1}{2k_1}\frac{d\mathbf{k}_2}{2k_2}\frac{d\mathbf{k}_3}{2k_3}\delta\left(\mathbf{k}+\mathbf{k}_1-\mathbf{k}_2-\mathbf{k}_3\right)\delta\left(k+k_1-k_2-k_3\right)\left(f^{+}_{\mathbf{k}}f^{-}_{\mathbf{k}_1}-f^{+}_{\mathbf{k}_2}f^{-}_{\mathbf{k}_3}\right). \quad (24)$$

In areas of phase space where the distribution function is sufficiently large, we can neglect the in-scattering terms compared to the out-scattering, as there is much greater phase space for scattering out of the narrow distribution than into it. The integral may then be evaluated analytically:

$$\begin{aligned}
S^{ph}_{\mathbf{k}}[f^{\pm}_{\mathbf{q}}] &= -\frac{2u_0^2}{9}\frac{1}{(2\pi)^{2d-1}}\frac{f^{+}_{\mathbf{k}}}{k}\int\frac{d\mathbf{k}_1}{2k_1}\frac{d\mathbf{k}_2}{2k_2}\frac{d\mathbf{k}_3}{2k_3}\delta\left(\mathbf{k}+\mathbf{k}_1-\mathbf{k}_2-\mathbf{k}_3\right)\delta\left(k+k_1-k_2-k_3\right)f^{-}_{\mathbf{k}_1}\\
&= -\frac{2u_0^2}{9}\frac{1}{(2\pi)^{2d-1}}\frac{f^{+}_{\mathbf{k}}}{k}\int\frac{d\mathbf{k}_1}{2k_1}\frac{d\mathbf{k}_2}{2k_2}\frac{d\mathbf{k}_3}{2k_3}\delta\left(\mathbf{k}+\mathbf{k}_1-\mathbf{k}_2-\mathbf{k}_3\right)\delta\left(k+k_1-k_2-k_3\right)f^{T}_{\mathbf{k}_1}\\
&= -\frac{2u_0^2}{9}\frac{1}{(2\pi)^{2d-1}}\frac{f^{+}_{\mathbf{k}}}{k}\int dk_2dk_3\frac{\pi^2}{k}f^{T}_{k_2+k_3-k}\mathrm{Min}\left(k,k_2,k_3,k_2+k_3-k\right)\\
&= -\frac{128\pi^4\epsilon^2}{25}\frac{1}{(2\pi)^5}\frac{f^{+}_{\mathbf{k}}}{k}\frac{\pi^2}{k}\frac{\pi^2}{6}kT^2\\
&= -\frac{2\pi^3\epsilon^2}{75}\frac{f^{+}_{\mathbf{k}}}{k}T^2, \qquad (25)
\end{aligned}$$

where $f^T$ is a thermal distribution, and we have used the identity

$$\int dk_1 g_{k_1}\int d\Omega_1 d\Omega_2 d\Omega_3\delta(k+k_1-k_2-k_3)\delta(\mathbf{k}+\mathbf{k}_1-\mathbf{k}_2-\mathbf{k}_3) = \frac{8\pi^2\mathrm{Min}\left(k,k_2,k_3,k_2+k_3-k\right)}{kk_2k_3(k_2+k_3-k)}g_{k_2+k_3-k}. \quad (26)$$

This should be compared with the scattering integral in the $1/N$ expansion[3], which can also be written as $\mathcal{S}[f_q]=-\Gamma_k f_k$. Here our phase-space argument for scattering out of the elongated distribution plays the same role as an argument about scattering out of the current carrying modes and into the remaining $N-2$ modes of the $1/N$ approach.

## VII. EXPANDING ABOUT A THERMAL DISTRIBUTION

We now consider the procedure of expanding about a thermal distribution at an effective temperature. This expansion does not converge and the procedure fails, but this gives important insight into the nature of the true solution.

Before solving the Boltzmann equation for the distribution function we must fix two parameters - the coefficient of the sink term $\alpha$, and the effective temperature $\tilde{T}$. By taking two moments of the Boltzmann equation we are able to obtain two equations which must be satisfied to enforce number and energy conservation (as in section IV, but with a different sink and distribution function, note that here we only require two moments as we only have two unknowns). These fix $\alpha$, the overall prefactor of the sink and $T_{eff}$ the effective temperature to be

$$\begin{aligned}
\alpha &= \frac{1}{32\zeta(3)T^4_{eff}},\\
T_{eff} &= \frac{45\zeta(3)}{\pi^5}\left(1+\frac{(2\pi)^3}{\sqrt{E}}\sigma_E\right)\sqrt{E}, \qquad (27)
\end{aligned}$$

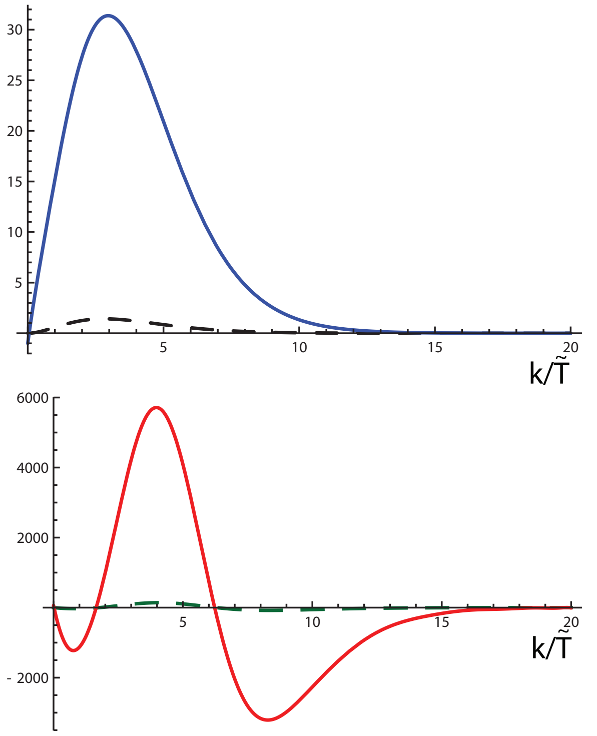


FIG. 1: Top: $(k/\tilde{T})^3 f_k^{T_{eff}}$ (dashed), $(k/\tilde{T})^3\epsilon^2\delta f^{A(1)}/\mathbf{k}\cdot\mathbf{E}$ (solid). Bottom: $(k/\tilde{T})^3\epsilon^2\delta f^{S(2)}$ (dashed) and $(k/\tilde{T})^3\epsilon^4\delta f^{A(2)}/\mathbf{k}\cdot\mathbf{E}$ (solid) as a function of $k/\tilde{T}$. Note that each term in the series grows.

where $\sigma_E$ is the electrical conductivity, which we will approximate to linear response order at this point. In fact the conductivity is itself a function of $T_{eff}$ and $\epsilon$. Eq.(27) is therefore a self-consistent, $\epsilon$-dependent equation for $T_{eff}$. We will later solve Eq.(27) for $T_{eff}$ in the hydrodynamic limit.

Having replaced the spatial gradients in the Boltzmann equation with a sink term representing scattering into the heat-carrying modes, we have a universal spatially homogeneous steady-state Boltzmann equation:

$$\pm\mathbf{E}\cdot\partial_{\mathbf{k}} f_{\mathbf{k}}^{\pm} \;=\; \mathcal{S}[f_{\mathbf{q}}^{\pm}] + G_{\mathbf{k}}, \qquad (28)$$

where $G_{\mathbf{k}} = g_{\mathbf{k}}^{source} - g_{\mathbf{k}}^{sink}$. The sink term is given by $g_{\mathbf{k}}^{sink} = \alpha v^y h_{\mathbf{k}}$, as in the highly-boosted case, but the zero-mode is the zero-mode of the scattering integral linearised about a thermal distribution $h_{\mathbf{k}} = v^y\partial_k f_k^T$. A formal solution of this equation may be obtained through an expansion in powers of $\epsilon$, which enters into the scattering integral. In order to solve Eq.(28) we expand the distribution function in devations from a thermal distribution function. This deviation is itself seperated into a term antisymmetric in both the momentum parallel to the applied electric field and the particle-hole channel index - $\delta f_{k_{||}}^A$, and a term symmetrical in both - $\delta f_k^S$:

$$f_{\mathbf{k}}^{\pm} \;=\; f_k^{T_{eff}} \pm \delta f_{k_{||}}^A + \delta f_k^S \qquad (29)$$

There is a linearised scattering integral for each of the symmetries of deviation: $\mathcal{S}$ is the scattering integral for the particle-hole antisymmetric, $k_{||}$ antisymmetric channel. This is the scattering integral which governs the electrical conductivity and was derived in[2,4]. $\mathcal{S}'$ is the particle-hole symmetric, $k_{||}$ symmetric scattering integral. This controls scattering into the symmetric part of the distribution and is derived along similar lines to the antisymmetric integral. This derivation is given in the appendix. The linearised scattering integrals have the form $\mathcal{S}_{k,q}\phi_q = -\epsilon^2 T\left(\int_q F_1(k,q)\phi_k + \int_q F_2(k,q)\phi_q\right)$, where $F_1$ and $F_2$ are lengthy functions of polylogarithms which are discussed further in the appendix.

The Boltzmann equation splits into two parts according to their symmetries:

$$\begin{aligned} \mathbf{E}\cdot\partial_{\mathbf{k}}(f_{\mathbf{k}}^{T_{eff}} + \delta f_k^S) \;&=\; \epsilon^2\mathcal{S}\delta f_{k_{||}}^A, \\ \mathbf{E}\cdot\partial_{\mathbf{k}}\delta f_{k_{||}}^A - G_{\mathbf{k}}(\mathcal{O}(\epsilon^{-2})) \;&=\; \epsilon^2\mathcal{S}'\delta f_k^S, \end{aligned} \qquad (30)$$

where we have explicitly included the $\epsilon$-dependence of the scattering integrals and of the source and sink terms. We note that although there is no explicit $\epsilon$ dependence in $G_{\mathbf{k}}$, in fact it enters through the effective temperature. The requirement of energy conservation shows that to be self-consistent, $G_{\mathbf{k}}$ must have the same $\epsilon$-dependence as the conductivity. We truncate the conductivity at linear-response order so $G_{\mathbf{k}}$ must be proportional to $\epsilon^{-2}$.

We can now proceed to expand the solutions for $\delta f_{k_{||}}^A$ and $\delta f_k^S$ in powers of $\epsilon$ to obtain the following expressions at order $\epsilon^{-2}$ and $\epsilon^{-4}$:

$$\begin{aligned} \delta f_{k_{||}}^A \;&=\; \delta f_{k_{||}}^{A(1)} + \delta f_{k_{||}}^{A(2)}, \\ \delta f_k^S \;&=\; \delta f_k^{S(1)}, \\ \delta f_{k_{||}}^{A(1)} \;&=\; \epsilon^{-2}\mathcal{S}^{-1}\mathbf{E}\cdot\partial_{\mathbf{k}} f_k^{T_{eff}}, && (31a) \\ \delta f_k^{S(2)} \;&=\; \epsilon^{-2}\mathcal{S}'^{-1}\left(G_{\mathbf{k}} + \epsilon^{-2}\mathbf{E}\cdot\partial_{\mathbf{k}} f_{k_{||}}^{A(1)}\right), && (31b) \\ \delta f_{k_{||}}^{A(2)} \;&=\; \epsilon^{-2}\mathcal{S}^{-1}\mathbf{E}\cdot\partial_{\mathbf{k}} f_k^{S(2)}. && (31c) \end{aligned}$$

The lowest order antisymmetric term $\delta f_{k_{||}}^{A(1)}$ is the linear response solution. This is the result that would be obtained by considering a weak electric field causing small deviations from the equilibrium distribution in the absence of any nonlinear effects such as pair-production. This was calculated by Damle and Sachdev[4] in their original formulation of the Boltzmann transport approach to the quantum critical point. There is no symmetric term of corresponding order; the first such non-equilibrium symmetric term occurs at order $\epsilon^{-4}$. The next order antisymmetric term is a function of this symmetric term. This antisymmetric term contributes to the conductivity.

The expansion of the Boltzmann equation will be controlled in the hydrodynamic limit where scattering is the most rapid process. Each term in the expansion comes with additional powers of $\epsilon^{-2}\mathcal{S}^{-1}$ which must therefore be small - corresponding to the hydrodynamic limit.

However, the Boltzmann equation is formally derived in the limit of $\epsilon$ small and so $\epsilon^{-1}$ large. This is the first indication that the expansion will not converge. For the present we assume the hydrodynamic limit in which case Eq.(27) for $T_{eff}$ reduces to $T_{eff} = 45\zeta(3)\sqrt{E}/\pi^5$.

It now remains to invert the scattering integrals numerically and obtain explicit results for the distribution function. We achieve this inversion by discretising the scattering integrals in a basis of Chebyshev polynomials and inverting the resulting matrices. This method achieves excellent agreement with the continuous integrals for only a modest number of Chebyshev polynomials. The results of this inversion are presented in Fig.(1). Each term in the expansion is substantially larger than the previous one. The expansion about an effective thermal distribution is therefore insufficient to describe the non-equilibrium state.

## Appendix A: Linearising the scattering integrals about a thermal distribution

We follow the linearization procedure of Refs(2,4). As stated in Section V the full collision term is:

$$\mathcal{S}_{\mathbf{q}}[f^{\pm}_{\mathbf{q}}, f^{\mp}_{\mathbf{q}}] \;=\; -\frac{2u_0^2}{9}\int d\underline{\mu}(\mathcal{F}^{out}_{\pm} - \mathcal{F}^{in}_{\pm}) \qquad \text{(A1)}$$

where

$$d\underline{\mu} \;=\; \frac{1}{2\epsilon_k}\left[\prod_{i=1}^{3}\frac{d^dk_i}{(2\pi)^d}\frac{1}{2\epsilon_{k_i}}\right](2\pi)^d\delta(\mathbf{k}+\mathbf{k}_1-\mathbf{k}_2-\mathbf{k}_3)(2\pi)\delta(\epsilon+\epsilon_1-\epsilon_2-\epsilon_3) \qquad \text{(A2)}$$

contains the product of three $d$-dimensional integral measures. We substitute the expanded form of the distribution function $f^{\pm} = f^T + \delta f^S \pm \delta f^A = f^T + \phi_S \pm \mathbf{k}\cdot\mathbf{E}\,\phi_A$, choosing a particular antisymmetric form for $\delta f^A$, and ignore terms of $\mathcal{O}(\delta^2)$. Using the identity $1 + f^T = e^{\beta\epsilon} f^T$ and interchanging $\mathbf{k}_2 \leftrightarrow \mathbf{k}_3$ in the last term, $(\mathcal{F}^{out}_{\pm} - \mathcal{F}^{in}_{\pm})$ can be simplified resulting in the linearised scattering integrals

$$\begin{aligned}
S_{\pm} \;&=\; \pm\left(-\frac{2u_0^2}{9}\right)\int d\underline{\mu}\,[-3\mathbf{k}\cdot\mathbf{E}\,\phi_A(k)\,T(k,k_1,k_2,k_3) + \mathbf{k}_1\cdot\mathbf{E}\,\phi_A(k_1)\,T(k_1,k,k_2,k_3) + 2\mathbf{k}_2\cdot\mathbf{E}\,\phi_A(k_2)\,T(k_2,k_3,k,k_1)]\,,\\
S'_{\pm} \;&=\; \left(-\frac{2u_0^2}{9}\right)\int d\underline{\mu}\,[-3\phi_S(k)\,T(k,k_1,k_2,k_3) - 3\phi_S(k_1)\,T(k_1,k,k_2,k_3) + 6\phi_S(k_2)\,T(k_2,k_3,k,k_1)]\,, \qquad \text{(A3)}
\end{aligned}$$

where $S_{\pm}$ acts on the fully antisymmetric deviation and $S'_{\pm}$ on the symmetric deviation, and

$$T(k,k_1,k_2,k_3) \;=\; \left(e^{k_2+k_3} - e^{k_1}\right) n_{\mathbf{k}_1} n_{\mathbf{k}_2} n_{\mathbf{k}_3}\delta(k+k_1-k_2-k_3). \qquad \text{(A4)}$$

We use $u_0 = 24/5\pi^2\epsilon$. Performing some of the integrals using the identities (C1), (C3), (C5) of Ref.(4) gives the antisymmetric linearised collision integral as

$$S_{\pm} \;=\; \pm\mathbf{k}\cdot\mathbf{E}\left(-\epsilon^2\int_0^{\infty} dk_1\,[F_1(k,k_1)\phi_A(k) + F_2(k,k_1)\phi_A(k_1)]\right), \qquad \text{(A5)}$$

where $F_1$ and $F_2$ are given in Ref.(2). We now go through the process in detail for the symmetric term, using a slightly more compact notation than that of Ref.(4).

Writing the measure $d^3k_i = k_i^2 dk_i d\Omega_i$ we can perform the angular integrals using the identity

$$\begin{aligned}
\tilde{I}(k,k_1,k_2,k_3) \;&=\; \int d\Omega_1 d\Omega_2 d\Omega_3 \delta^3(\mathbf{k}+\mathbf{k}_1-\mathbf{k}_2-\mathbf{k}_3)\delta(k+k_1-k_2-k_3)\\
&=\; \frac{8\pi^2}{kk_1k_2k_3}\mathrm{Min}(k,k_1,k_2,k_3)\delta(k+k_1-k_2-k_3), \qquad \text{(A6)}
\end{aligned}$$

Where $\mathrm{Min}(k,k_1,k_2,k_3)$ gives the smallest of $k, k_1, k_2, k_3$ or 0 if this is negative. Interchanging $k_1 \leftrightarrow k_3$ in the first and last terms of (A3), we use the identity (A6). Here we note that $T$ inherits the symmetries of the measure, when integrated over $k$ it is invariant under the following exchanges of terms in the argument: $1 \leftrightarrow 2, 3 \leftrightarrow 4, (1,2) \leftrightarrow (3,4)$. The scattering integral may now be written

$$S'_{\pm} \;=\; -\epsilon^2\left(\int_0^{\infty} dk_1 F_1(k,k_1)\phi_S(k) + \int_0^{\infty} dk_1 F_3^a(k,k_1)\phi_S(k_1) + \int_0^{\infty} dk_1 F_3^b(k,k_1)\phi_S(k_1)\right), \qquad \text{(A7)}$$

and (interchanging $k_1, k_2$ in the last term)

$$\begin{aligned} F_1(k,k_1) &= \frac{-6\pi}{25k^2}\int_0^\infty dk_2\, T(k,k_1+k_2-k,k_1,k_2)\mathrm{Min}(k,k_1+k_2-k,k_2,k_1), \\ F_3^a(k,k_1) &= \frac{12\pi}{25k^2}\int_0^\infty dk_2\, T(k_1,k_2,k,k_1+k_2-k)\mathrm{Min}(k,k_1+k_2-k,k_1,k_2), \\ F_3^b(k,k_1) &= \frac{-6\pi}{25k^2}\int_0^\infty dk_2\, T(k_1,k,k_2,k+k_1-k_2)\mathrm{Min}(k,k_1,k_2,k+k_1-k_2). \end{aligned} \tag{A8}$$

We note that $F_1$ is identical to that found in Ref.(4) and $F_3^a$ can be re-expressed in terms of $F_1$:

$$F_3^a(k,k_1) = 2\left(\frac{n(k)}{n(k_1)}\right)^2 \frac{n(k_1-k)}{n(k-k_1)} F_1(k,k_1). \tag{A9}$$

These integrals may be performed to give:

$$F_1(k,k_1) = \frac{6\pi}{25k^2}\frac{n(k_1)n(k-k_1)}{n(k)}T^2\Gamma(2)\left[\Theta(k-k_1)\mu_2(k,k_1)-\Theta(k_1-k)\mu_2(k_1,k)\right], \tag{A10}$$

where

$$\mu_2(k,k_1) = -\mathrm{Li}_2\left(e^{-(k-k_1)/T}\right)+\mathrm{Li}_2\left(e^{-k/T}\right)+\mathrm{Li}_2(1)-\mathrm{Li}_2\left(e^{-k_1/T}\right), \tag{A11}$$

and

$$\begin{aligned} F_3^b(k,k_1) &= -\frac{6\pi}{25k^2}\frac{n(k)n(k+k_1)}{n(k_1)}e^{\beta k}T^2\Gamma(2) \\ &\times\left[\mathrm{Li}_2\left(e^{(k+k_1)/T}\right)-\mathrm{Li}_2\left(e^{k/T}\right)-\mathrm{Li}_2\left(e^{k_1/T}\right)+\mathrm{Li}_2\left(e^{-k/T}\right)+\mathrm{Li}_2\left(e^{-k_1/T}\right)-\mathrm{Li}_2\left(e^{-(k+k_1)/T}\right)\right]. \end{aligned} \tag{A12}$$

[1] A. M. Tremblay, B. Patton, P. C. Martin, and P. F. Maldague, Phys. Rev. A **19**, 1721 (1979).
[2] M. J. Bhaseen, A. G. Green, and S. L. Sondhi, Phys. Rev. B **79**, 094502 (2009).
[3] A. G. Green and S. L. Sondhi, Phys. Rev. Lett. **95**, 267001 (2005).
[4] K. Damle and S. Sachdev, Phys. Rev. B **56**, 8714 (1997).
[5] The symmetrisation is performed in order to simplify integrals over the source term. We do not expect this to effect the results as we anticipate a solution elongated along the field direction, regardless of the symmetry of the source term.
